# Supplementary material for: Prediction of quaternary hydrides based on densest ternary sphere packings
Source: arXiv:2206.04971 source file (2022-06-10)
Supplement: Supplementary file 1 [file SupplementalMaterials.pdf]

# Supplemental materials for prediction of quaternary hydrides based on densest ternary sphere packings

The phonon dispersions of the 16 kinds of the (12-1-2-1)$_V$-type hydrides listed in Table II of the main article are shown in Figs. 1 and 2, and the band structures and DOS of them are shown in Figs. 3 and 4. Note that $H_{12}ScLa_2Zr$ and $H_{12}TiSc_2Sr$, which have the SFEs less than $-10.0$ eV/f.u. and exhibit no spin polarization, are excluded from the table, since their phonon dispersions show the dynamic instability. The NPTMD of $H_{12}ScLa_2Zr$ also indicates the dynamic instability, but the NPTMD of $H_{12}TiSc_2Sr$ indicates the dynamic stability. Tables I and II list the 167 kinds of the (12-1-2-1)$_V$-type hydrides that show the dynamic stability in NVTMDs, and have the SFEs more than $-10.0$ eV/f.u., and exhibit no spin polarization. Table III lists the 66 kinds of the (12-1-2-1)$_V$-type hydrides that also show the dynamic stability in NVTMDs but exhibit spin polarization.

The phonon dispersion and band structure of $H_{12}TiSc_2Cs$ are shown in Figs. 5 and 6, respectively.

The phonon dispersions of the six kinds of the (12-1-3-1)-type hydrides listed in Table III of the main article are shown in Fig. 7, and the band structures and DOS of them are shown in Fig. 8. We exclude $H_{12}KSc_3Cs$ and $H_{12}TiNi_3La$, which have the SEFs less than $-5.0$ eV/f.u. and exhibit no spin polarization, from Table III of the main article, since both the phonon dispersions and NPTMDs indicate their dynamic instability. Besides, we did not calculate the phonon dispersion of $H_{12}LiRu_3La$, which has the SEF of $-5.36$ eV/f.u. and exhibit no spin polarization, since it has a large structural distortion. However, the NPTMD of the hydride indicates the dynamical stability. Table IV lists the 62 kinds of the (12-1-3-1)-type hydrides that show the dynamic stability in NVTMDs, and have the SFEs more than $-5.0$ eV/f.u., and exhibit no spin polarization. Table V lists the 36 kinds of the (12-1-3-1)-type hydrides that show the dynamic stability in NVTMDs but exhibit spin polarization.

As shown in Table I of the main article, 49 kinds of atoms substitute the spheres in the PDTSPs. The pseudoatomic orbital basis functions in the OpenMX code for the 49 kinds of atoms are listed in Table VI. The basis functions are expanded by linear combination of multiple pseudoatomic orbitals generated using a confinement scheme [1, 2]. The symbol of each basis denotes the element, cutoff radius (Bohr units), and the allocated radial functions of $s$, $p$, $d$, and $f$ orbitals. We use the Quick Basis in geometrical optimizations, NVTMDs, and NPTMDs. On the other hand, we use the Standard Basis in calculating the SFEs and phonon dispersions.

[1] T. Ozaki, Phys. Rev. B **67**, 155108 (2003).
[2] T. Ozaki and H. Kino, Phys. Rev. B **69**, 195113 (2004).

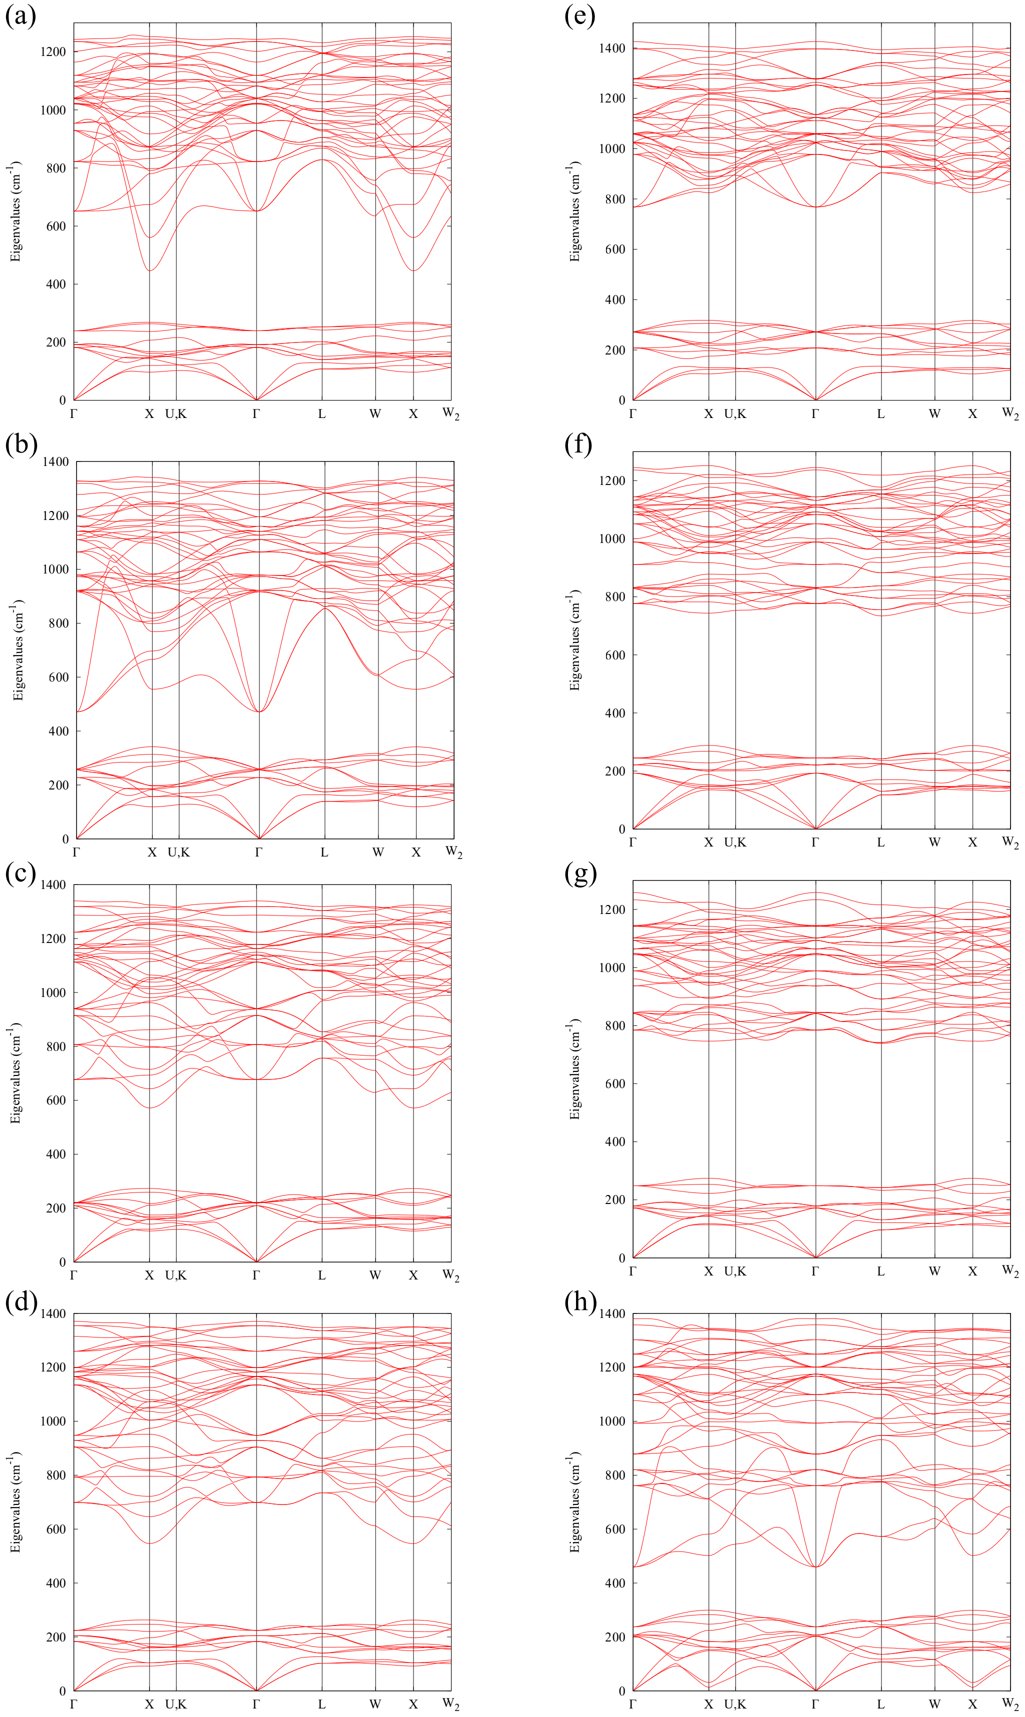


FIG. 1. The phonon dispersions of the (12-1-2-1)$_V$-type hydrides. Note that the force constants for phonon dispersions are calculated after symmetrization to have the $Fm\bar{3}$ symmetry. (a) $H_{12}ScY_2La$. (b) $H_{12}ScSc_2Y$. (c) $H_{12}ScY_2Zr$. (d) $H_{12}ScY_2Hf$. (e) $H_{12}ScSc_2Hf$. (f) $H_{12}ScY_2Ca$. (g) $H_{12}ScY_2Sr$. (h) $H_{12}TiY_2Ca$.

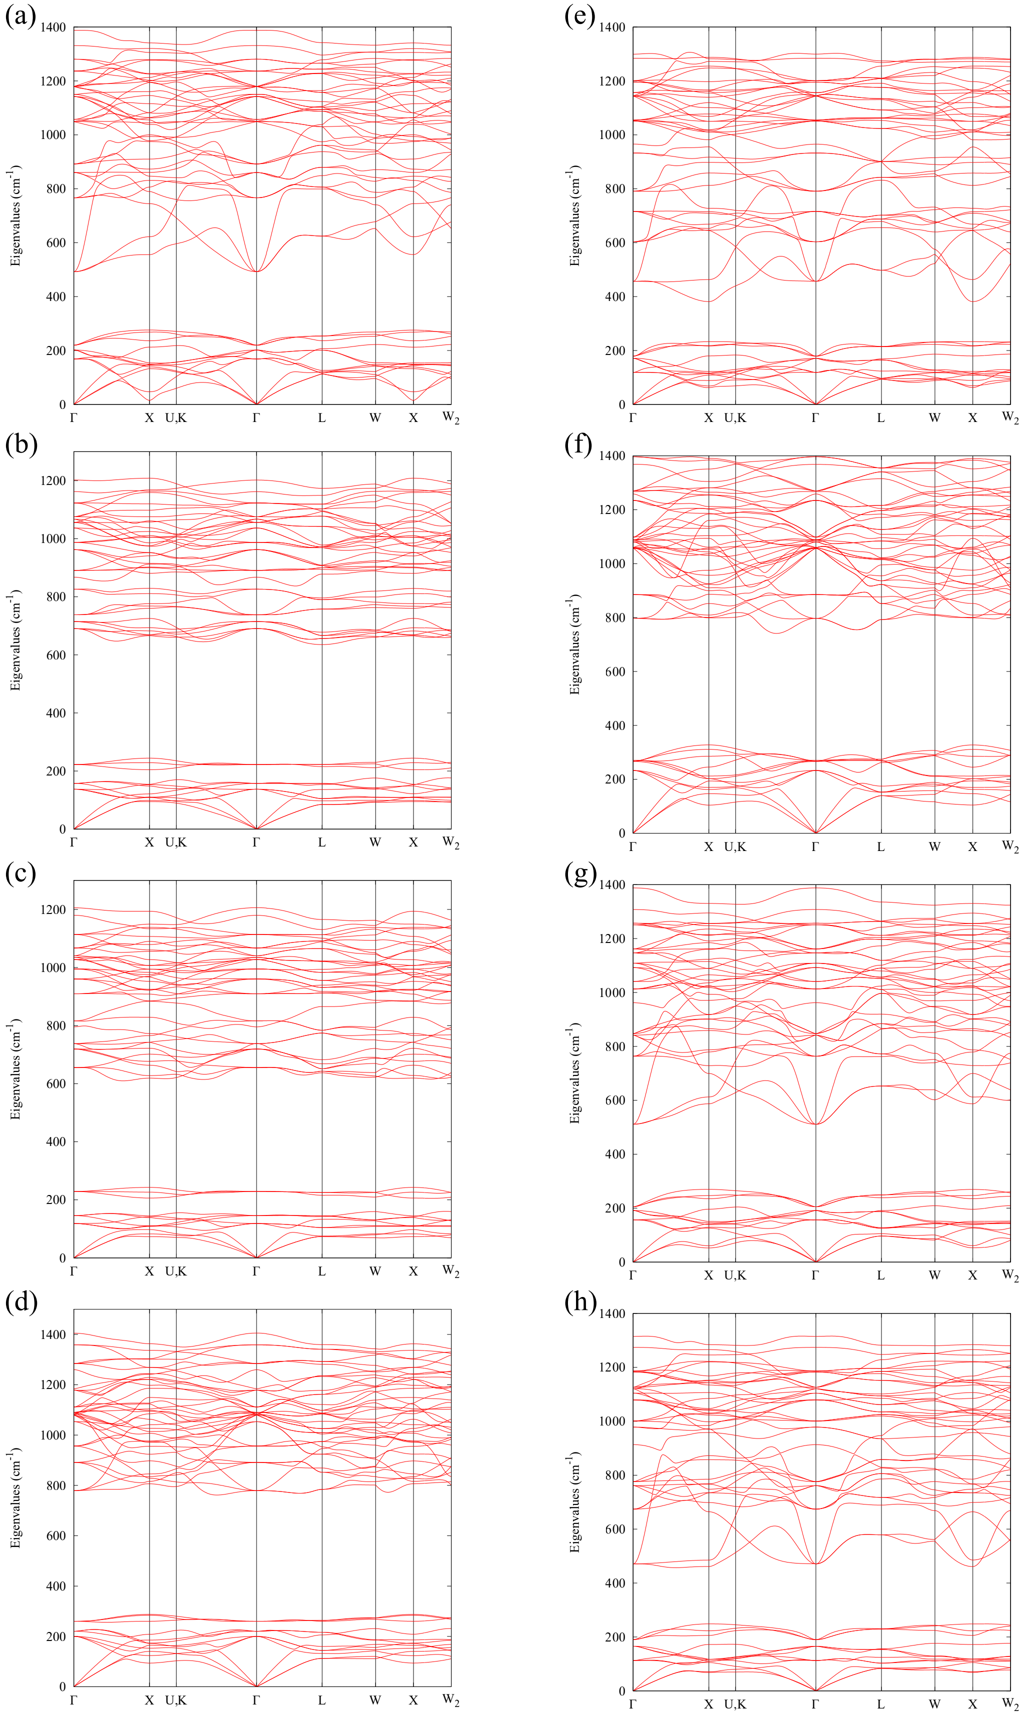


FIG. 2. The phonon dispersions of states of the $(12\text{-}1\text{-}2\text{-}1)_V$-type hydrides. Note that the force constants for phonon dispersions are calculated after symmetrization to have the $Fm\bar{3}$ symmetry. (a) $H_{12}TiY_2Sr$. (b) $H_{12}ScLa_2Sr$. (c) $H_{12}ScLa_2Ba$. (d) $H_{12}CaZr_2Zr$. (e) $H_{12}TiLa_2Sr$. (f) $H_{12}TiSc_2Zr$. (g) $H_{12}TiY_2Ba$. (h) $H_{12}TiLa_2Ba$.

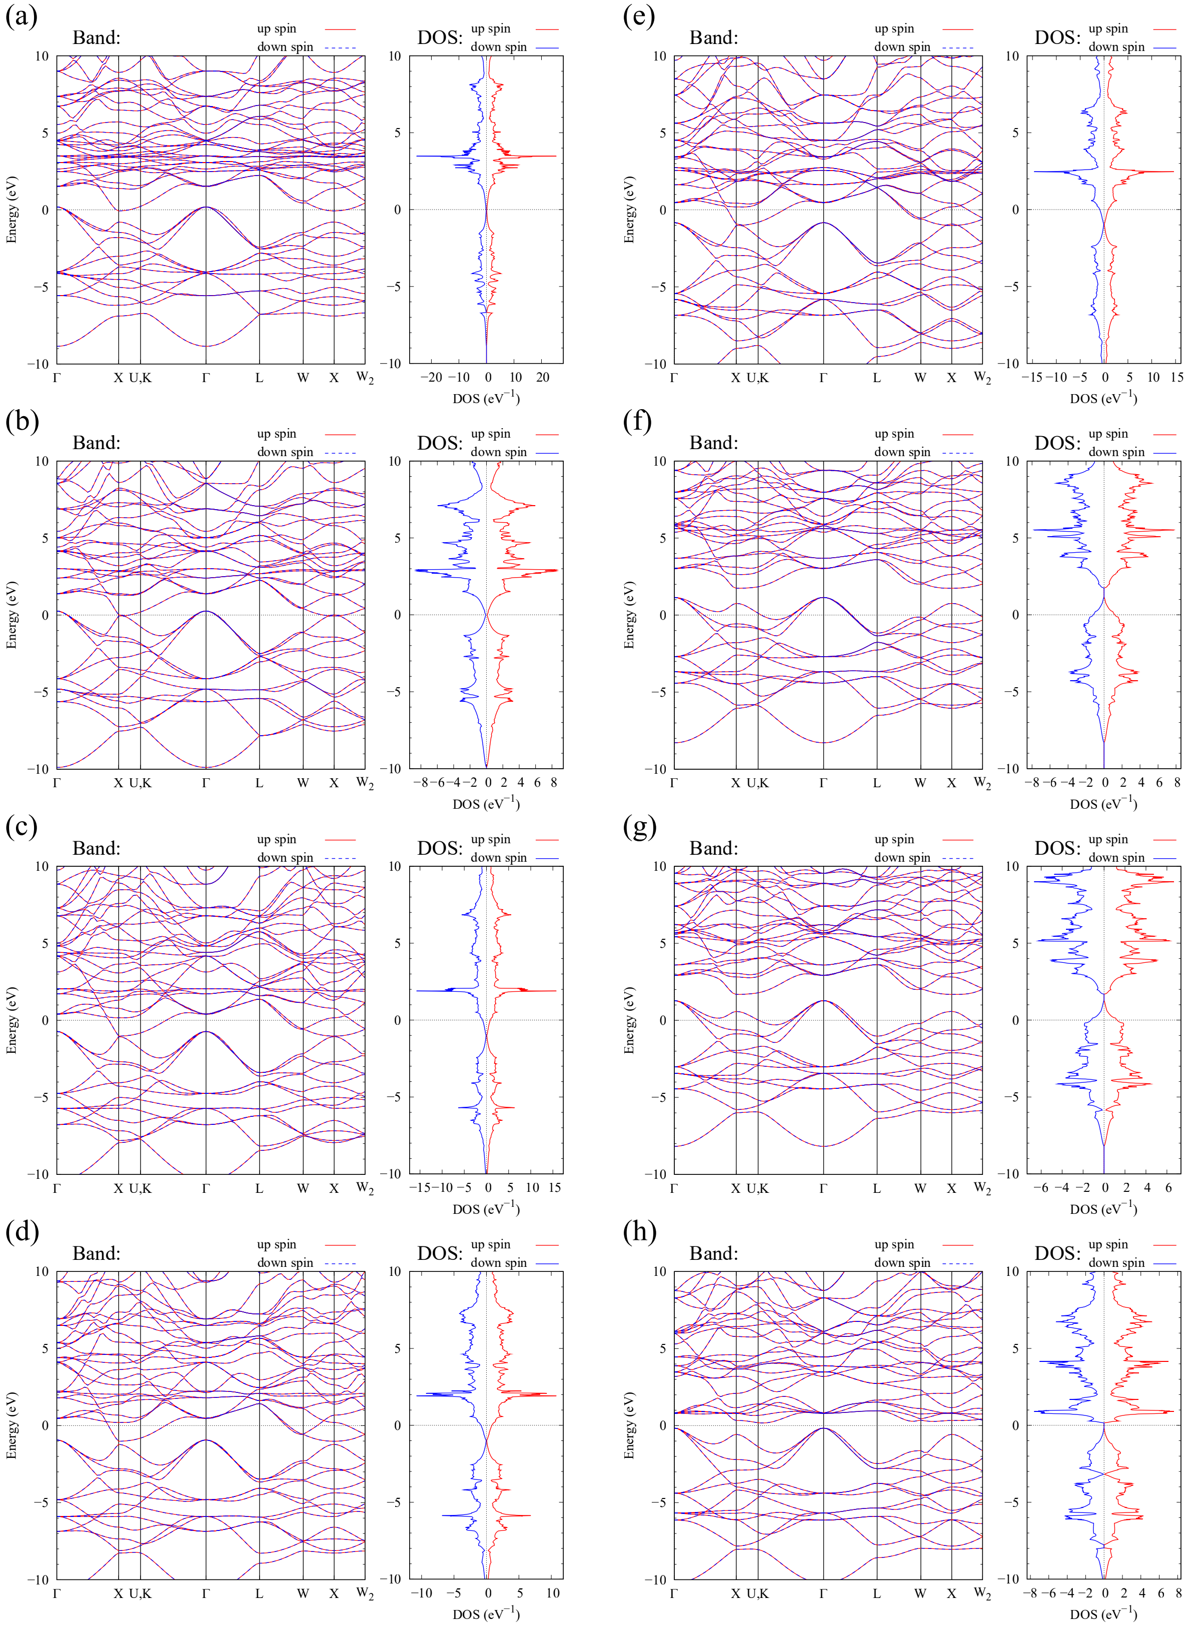


FIG. 3. The bands and DOS of the (12-1-2-1)$_V$-type hydrides. (a) $H_{12}ScY_2La$. (b) $H_{12}ScSc_2Y$. (c) $H_{12}ScY_2Zr$. (d) $H_{12}ScY_2Hf$. (e) $H_{12}ScSc_2Hf$. (f) $H_{12}ScY_2Ca$. (g) $H_{12}ScY_2Sr$. (h) $H_{12}TiY_2Ca$.

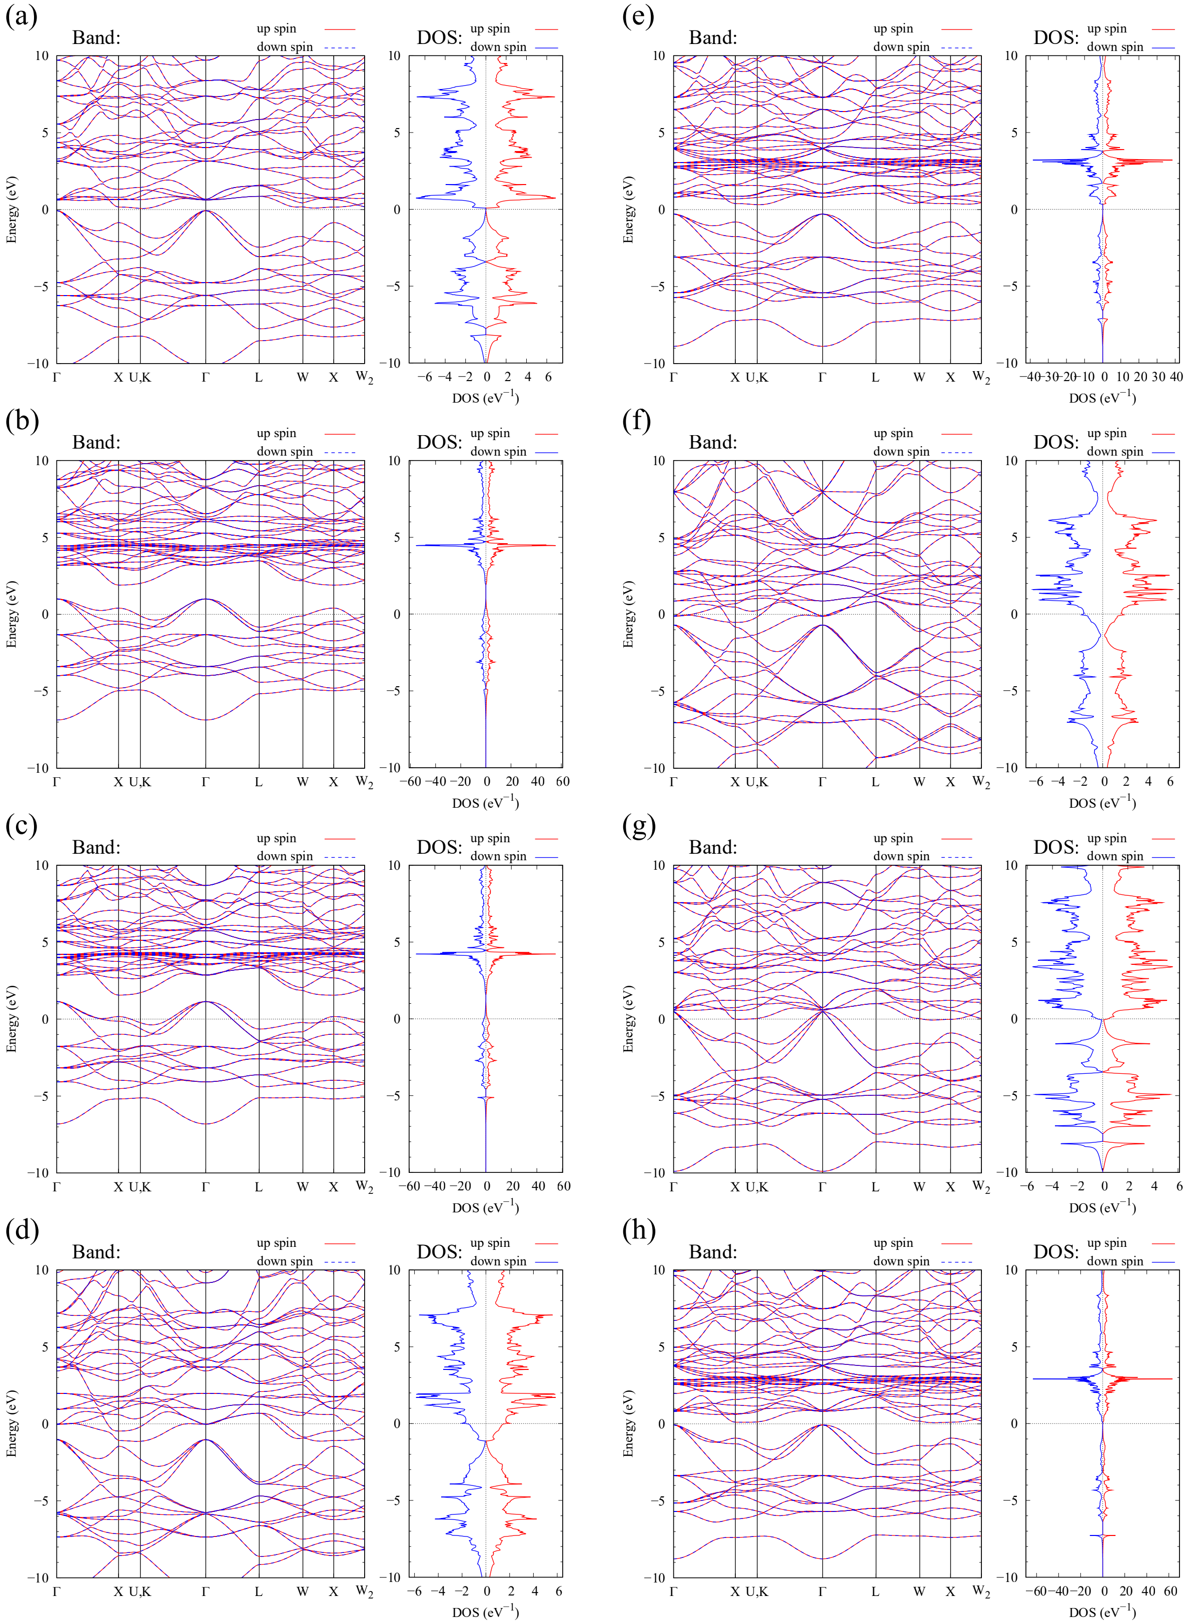


FIG. 4. The bands and DOS of the (12-1-2-1)$_V$-type hydrides. (a) $H_{12}TiY_2Sr$. (b) $H_{12}ScLa_2Sr$. (c) $H_{12}ScLa_2Ba$. (d) $H_{12}CaZr_2Zr$. (e) $H_{12}TiLa_2Sr$. (f) $H_{12}TiSc_2Zr$. (g) $H_{12}TiY_2Ba$. (h) $H_{12}TiLa_2Ba$.

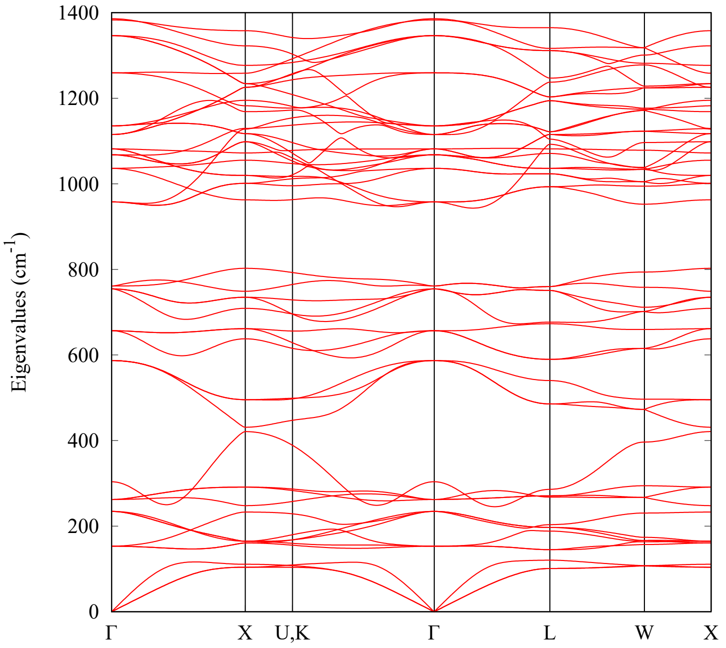


FIG. 5. The phonon dispersion of $H_{12}TiSc_2Cs$. Note that the force constant for the phonon dispersion is calculated after symmetrization to have the $Fm\bar{3}m$ symmetry.

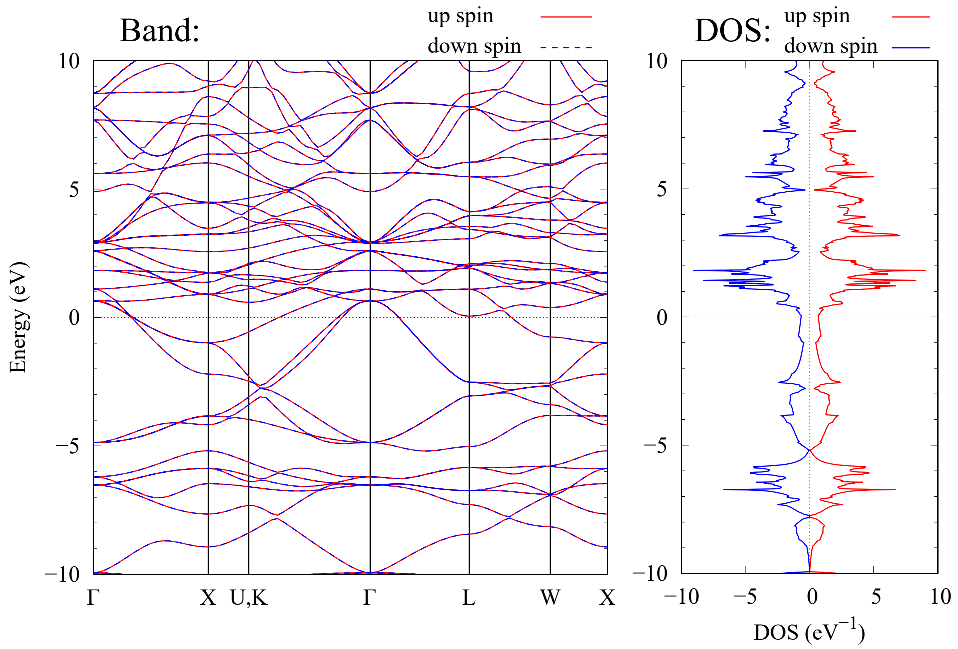


FIG. 6. The band and DOS of $H_{12}TiSc_2Cs$.

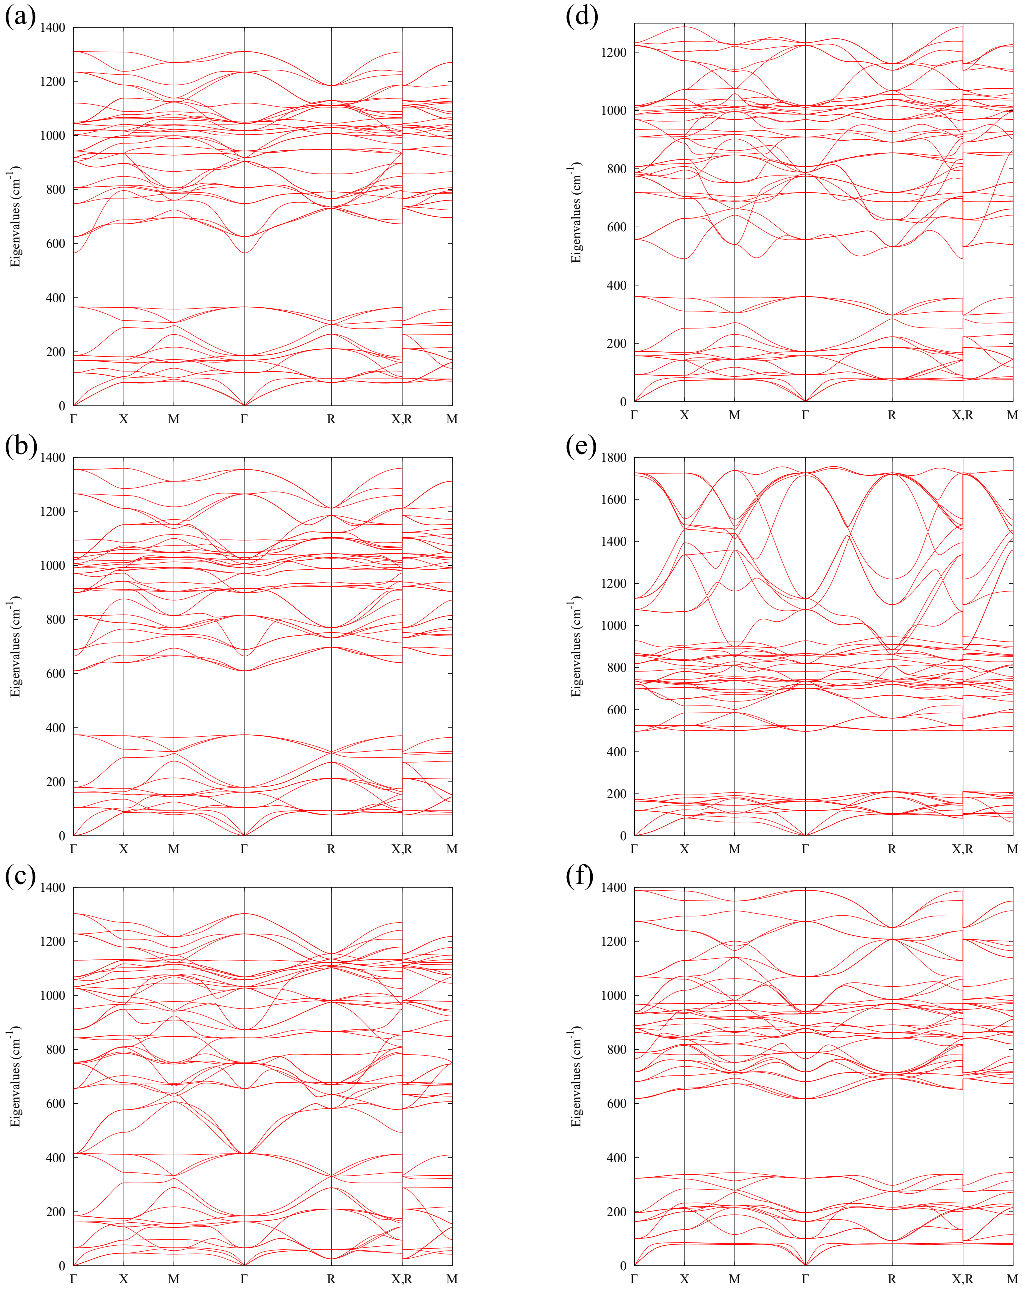


FIG. 7. The phonon dispersions of the (12-1-3-1)-type hydrides. Note that the force constants for phonon dispersions are calculated after symmetrization to have the $Pm\bar{3}m$ symmetry. (a) $H_{12}TiNi_3Ba$. (b) $H_{12}TiNi_3Sr$. (c) $H_{12}ScNi_3La$. (d) $H_{12}ScPd_3Ba$. (e) $H_{12}LiRu_3Ba$. (f) $H_{12}TiPd_3Ba$.

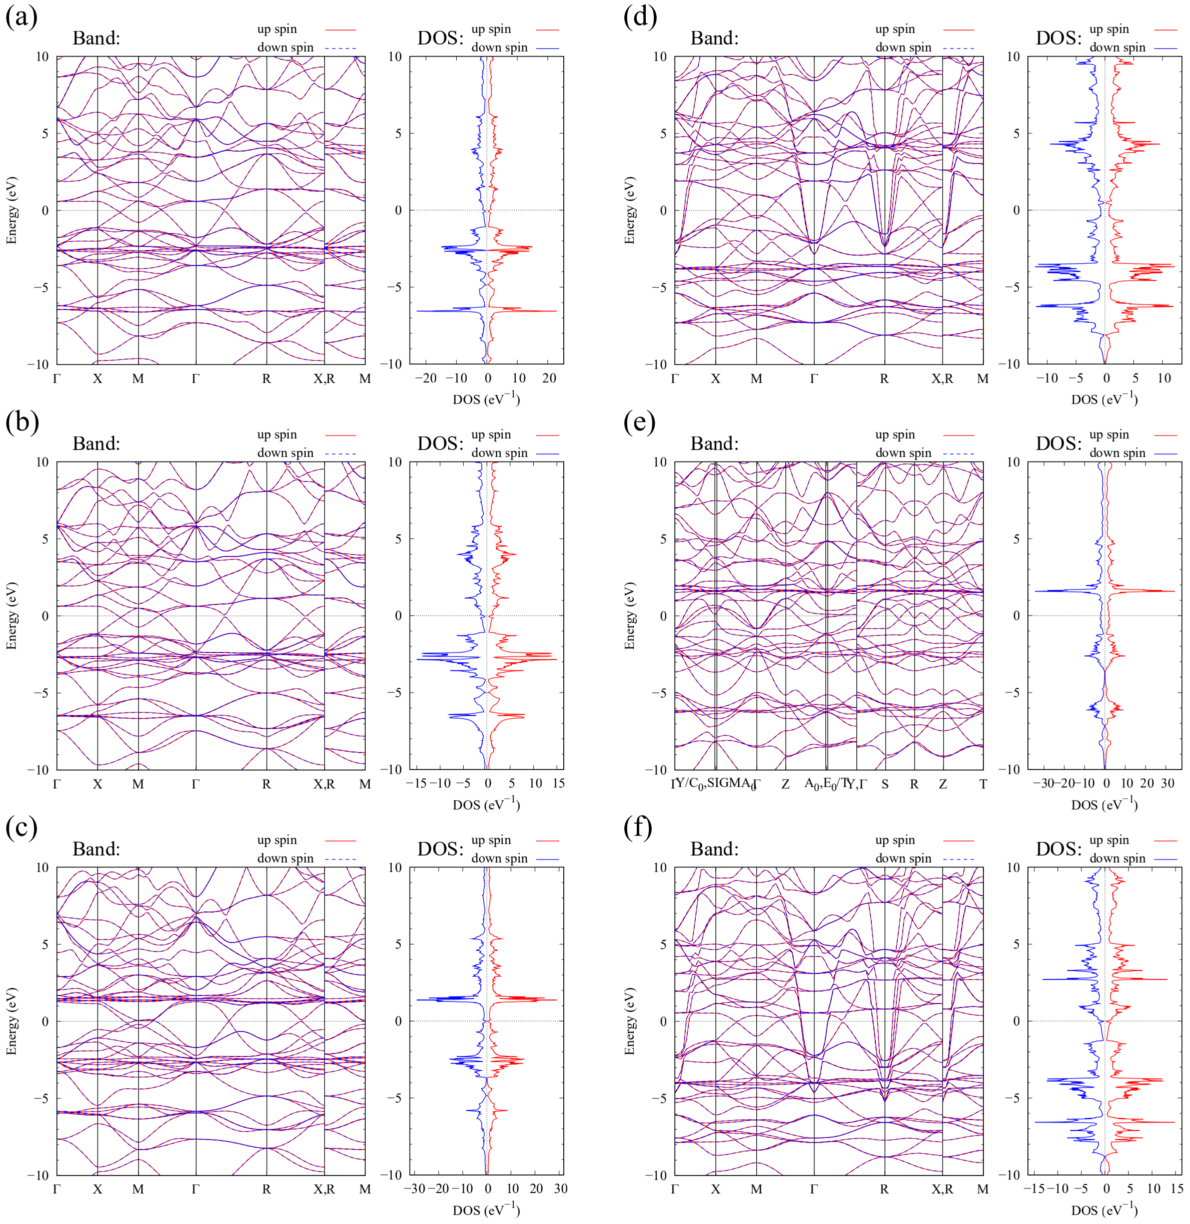


FIG. 8. The bands and DOS of the (12-1-3-1)-type hydrides. (a) $H_{12}TiNi_3Ba$. (b) $H_{12}TiNi_3Sr$. (c) $H_{12}ScNi_3La$. (d) $H_{12}ScPd_3Ba$. (e) $H_{12}LiRu_3Ba$. (f) $H_{12}TiPd_3Ba$.

TABLE I. List of the 111 kinds of the (12-1-2-1)$_V$-type hydrides which have the SEFs between −10.00 eV/f.u and −5.00 eV/f.u. and no spin polarization. The hydrides show the dynamical stabilities in NVTMDs.

| SEFs (eV/f.u.) | Material names | SEFs (eV/f.u.) | Material names |
|---|---|---|---|
| −9.89 | $H_{12}TiLa_2La$ | −7.00 | $H_{12}TiZr_2Rb$ |
| −9.83 | $H_{12}TiLa_2Ca$ | −6.99 | $H_{12}LiTi_2Hf$ |
| −9.77 | $H_{12}TiY_2Hf$ | −6.99 | $H_{12}ScSc_2In$ |
| −9.62 | $H_{12}ScY_2Ta$ | −6.88 | $H_{12}VSc_2Rb$ |
| −9.53 | $H_{12}ScSc_2Nb$ | −6.82 | $H_{12}ScHf_2Ag$ |
| −9.45 | $H_{12}ScZr_2Ti$ | −6.81 | $H_{12}ScHf_2Pd$ |
| −9.45 | $H_{12}TiZr_2Sc$ | −6.80 | $H_{12}AlZr_2Sc$ |
| −9.38 | $H_{12}MgSc_2Zr$ | −6.78 | $H_{12}TiSc_2Cd$ |
| −9.38 | $H_{12}ScY_2Nb$ | −6.78 | $H_{12}TiHf_2Nb$ |
| −9.36 | $H_{12}TiZr_2Y$ | −6.76 | $H_{12}ScZr_2Cd$ |
| −9.23 | $H_{12}TiZr_2Ca$ | −6.74 | $H_{12}LiTi_2Y$ |
| −9.11 | $H_{12}TiY_2K$ | −6.71 | $H_{12}TiZr_2Pd$ |
| −9.11 | $H_{12}LiHf_2Sc$ | −6.71 | $H_{12}ScZr_2Zn$ |
| −9.10 | $H_{12}NaZr_2Sc$ | −6.71 | $H_{12}TiSc_2Ga$ |
| −9.09 | $H_{12}LiZr_2Sc$ | −6.63 | $H_{12}TiSc_2Zn$ |
| −8.97 | $H_{12}LiY_2Zr$ | −6.60 | $H_{12}ScY_2Hg$ |
| −8.91 | $H_{12}TiY_2Rb$ | −6.53 | $H_{12}ScZr_2Ga$ |
| −8.87 | $H_{12}TiLa_2Rb$ | −6.51 | $H_{12}TiHf_2Pd$ |
| −8.87 | $H_{12}MgY_2Sc$ | −6.49 | $H_{12}TiLa_2Hg$ |
| −8.83 | $H_{12}TiLa_2Cs$ | −6.43 | $H_{12}TiSc_2In$ |
| −8.76 | $H_{12}MgZr_2Y$ | −6.42 | $H_{12}ScHf_2Cd$ |
| −8.76 | $H_{12}LiZr_2Y$ | −6.36 | $H_{12}ScZr_2Au$ |
| −8.74 | $H_{12}TiLa_2K$ | −6.32 | $H_{12}ScZr_2Ge$ |
| −8.63 | $H_{12}LiZr_2Zr$ | −6.28 | $H_{12}MgY_2Ba$ |
| −8.63 | $H_{12}TiZr_2Sr$ | −6.22 | $H_{12}TiSc_2Hg$ |
| −8.59 | $H_{12}MgSc_2Ti$ | −6.18 | $H_{12}VY_2Te$ |
| −8.56 | $H_{12}MgY_2La$ | −6.16 | $H_{12}ScHf_2Au$ |
| −8.53 | $H_{12}TiY_2Cs$ | −6.14 | $H_{12}MgSc_2Sr$ |
| −8.37 | $H_{12}MgSc_2Y$ | −6.13 | $H_{12}LiHf_2Sr$ |
| −8.37 | $H_{12}TiSc_2K$ | −6.02 | $H_{12}ScZr_2Hg$ |
| −8.36 | $H_{12}LiHf_2Zr$ | −6.02 | $H_{12}ScHf_2Ge$ |
| −8.15 | $H_{12}MgLa_2La$ | −6.01 | $H_{12}TiZr_2Ag$ |
| −8.14 | $H_{12}TiSc_2Rb$ | −5.99 | $H_{12}TiZr_2Ga$ |
| −8.11 | $H_{12}TiCa_2Sr$ | −5.85 | $H_{12}TiZr_2Sn$ |
| −7.99 | $H_{12}LiZr_2Ti$ | −5.81 | $H_{12}TiSc_2Sb$ |
| −7.91 | $H_{12}ScHf_2Nb$ | −5.72 | $H_{12}TiZr_2Zn$ |
| −7.85 | $H_{12}LiHf_2Ti$ | −5.70 | $H_{12}TiZr_2Cd$ |
| −7.72 | $H_{12}LiY_2Sc$ | −5.69 | $H_{12}TiHf_2Ag$ |
| −7.64 | $H_{12}AlSc_2Y$ | −5.69 | $H_{12}AlY_2Ba$ |
| −7.63 | $H_{12}MgZr_2Sr$ | −5.69 | $H_{12}TiHf_2Ga$ |
| −7.62 | $H_{12}TiZr_2K$ | −5.69 | $H_{12}ScHf_2Hg$ |
| −7.55 | $H_{12}ScY_2In$ | −5.66 | $H_{12}TiHf_2Cu$ |
| −7.55 | $H_{12}LiZr_2La$ | −5.66 | $H_{12}TiZr_2Ge$ |
| −7.46 | $H_{12}MgSc_2La$ | −5.55 | $H_{12}CrY_2Te$ |
| −7.21 | $H_{12}LiTi_2Sc$ | −5.50 | $H_{12}TiZr_2Au$ |
| −7.21 | $H_{12}LiHf_2La$ | −5.49 | $H_{12}TiHf_2Zn$ |
| −7.18 | $H_{12}VSc_2K$ | −5.43 | $H_{12}TiZr_2In$ |
| −7.18 | $H_{12}TiY_2Cd$ | −5.32 | $H_{12}TiZr_2Hg$ |
| −7.16 | $H_{12}AlSc_2Zr$ | −5.31 | $H_{12}TiZr_2Te$ |
| −7.15 | $H_{12}MgY_2Ca$ | −5.31 | $H_{12}TiHf_2Ge$ |
| −7.13 | $H_{12}ScY_2Cd$ | −5.30 | $H_{12}TiZr_2Sb$ |
| −7.07 | $H_{12}TiZr_2Nb$ | −5.29 | $H_{12}TiHf_2Cd$ |
| −7.03 | $H_{12}TiZr_2Ta$ | −5.05 | $H_{12}VSc_2Te$ |
| −7.02 | $H_{12}ScZr_2Pd$ | −5.05 | $H_{12}TiTi_2Pd$ |
| −7.01 | $H_{12}ScZr_2Ag$ | −5.02 | $H_{12}VSc_2In$ |
| −7.00 | $H_{12}TiY_2In$ | | |

TABLE II. List of the 56 kinds of the $(12\text{-}1\text{-}2\text{-}1)_V$-type hydrides which have the SEFs between −5.00 eV/f.u and 0.00 eV/f.u. and no spin polarization. The hydrides show the dynamical stabilities in NVTMDs.

| SEFs (eV/f.u.) | Material names | SEFs (eV/f.u.) | Material names |
|---|---|---|---|
| −4.92 | $H_{12}VBa_2Rb$ | −3.92 | $H_{12}MgZr_2Ag$ |
| −4.91 | $H_{12}TiHf_2Hg$ | −3.86 | $H_{12}MgHf_2Ge$ |
| −4.88 | $H_{12}TiHf_2Te$ | −3.85 | $H_{12}LiZr_2Cd$ |
| −4.81 | $H_{12}CrSc_2Se$ | −3.81 | $H_{12}VHf_2Cd$ |
| −4.80 | $H_{12}VSc_2Sb$ | −3.76 | $H_{12}MgZr_2Hg$ |
| −4.74 | $H_{12}VZr_2Ga$ | −3.66 | $H_{12}AlSc_2In$ |
| −4.60 | $H_{12}VZr_2Te$ | −3.64 | $H_{12}TiTi_2Au$ |
| −4.58 | $H_{12}MgZr_2Ga$ | −3.62 | $H_{12}LiHf_2Cd$ |
| −4.52 | $H_{12}MgHf_2Ga$ | −3.60 | $H_{12}VHf_2Hg$ |
| −4.48 | $H_{12}TiTi_2Zn$ | −3.52 | $H_{12}LiHf_2Ge$ |
| −4.46 | $H_{12}CrSc_2Te$ | −3.43 | $H_{12}LiZr_2As$ |
| −4.45 | $H_{12}VZr_2As$ | −3.37 | $H_{12}AlZr_2Ag$ |
| −4.38 | $H_{12}VHf_2Ga$ | −3.31 | $H_{12}VTi_2Ga$ |
| −4.32 | $H_{12}TiTi_2Ga$ | −3.29 | $H_{12}TiTi_2Hg$ |
| −4.28 | $H_{12}VZr_2Au$ | −3.21 | $H_{12}VTi_2Zn$ |
| −4.28 | $H_{12}VZr_2Cd$ | −3.18 | $H_{12}AlHf_2Ag$ |
| −4.27 | $H_{12}TiTi_2Ag$ | −3.16 | $H_{12}AlZr_2Ge$ |
| −4.26 | $H_{12}VZr_2Sb$ | −3.13 | $H_{12}LiHf_2Sb$ |
| −4.23 | $H_{12}LiHf_2Ga$ | −3.05 | $H_{12}AlZr_2In$ |
| −4.13 | $H_{12}LiZr_2In$ | −2.87 | $H_{12}LiHf_2Hg$ |
| −4.12 | $H_{12}VZr_2Hg$ | −2.84 | $H_{12}VTi_2Ge$ |
| −4.08 | $H_{12}VHf_2As$ | −2.55 | $H_{12}VTi_2Au$ |
| −4.07 | $H_{12}VHf_2Te$ | −2.33 | $H_{12}VTi_2Hg$ |
| −4.07 | $H_{12}MgZr_2Ge$ | −2.33 | $H_{12}VTi_2Sb$ |
| −4.05 | $H_{12}TiTi_2Cd$ | −2.08 | $H_{12}LiTi_2Ge$ |
| −4.01 | $H_{12}MgHf_2In$ | −1.70 | $H_{12}CrTi_2Cd$ |
| −4.00 | $H_{12}LiHf_2In$ | −1.37 | $H_{12}CrTi_2Hg$ |
| −3.94 | $H_{12}VHf_2Au$ | −1.34 | $H_{12}AlTi_2Ge$ |

TABLE III. List of the 66 kinds of the (12-1-2-1)$_V$-type hydrides which have the SEFs between −10.00 eV/f.u and 0.00 eV/f.u. and spin polarizations. The hydrides show the dynamical stabilities in NVTMDs.

| SEFs (eV/f.u.) | Material names | SEFs (eV/f.u.) | Material names |
|---|---|---|---|
| −10.78 | $H_{12}TiY_2Y$ | −4.95 | $H_{12}VHf_2Pd$ |
| −10.56 | $H_{12}TiY_2La$ | −4.58 | $H_{12}VZr_2Sn$ |
| −10.52 | $H_{12}TiSc_2Sc$ | −4.56 | $H_{12}MgHf_2Sn$ |
| −10.38 | $H_{12}ScY_2Ti$ | −4.47 | $H_{12}LiHf_2Sn$ |
| −10.38 | $H_{12}TiY_2Sc$ | −4.43 | $H_{12}VZr_2Ag$ |
| −9.96 | $H_{12}TiSc_2La$ | −4.41 | $H_{12}VZr_2Ge$ |
| −9.23 | $H_{12}TiHf_2Sc$ | −4.39 | $H_{12}VHf_2Sn$ |
| −8.80 | $H_{12}TiZr_2Zr$ | −4.28 | $H_{12}VHf_2Rb$ |
| −8.72 | $H_{12}MgHf_2Sc$ | −4.27 | $H_{12}VZr_2Cs$ |
| −8.49 | $H_{12}LiHf_2Hf$ | −4.25 | $H_{12}AlSc_2Sn$ |
| −8.38 | $H_{12}VSc_2Y$ | −4.24 | $H_{12}LiZr_2Sn$ |
| −8.36 | $H_{12}TiHf_2Hf$ | −4.20 | $H_{12}VTi_2K$ |
| −8.27 | $H_{12}ScY_2Sn$ | −4.19 | $H_{12}VZr_2In$ |
| −8.24 | $H_{12}VY_2La$ | −4.10 | $H_{12}VHf_2Zn$ |
| −8.14 | $H_{12}VSc_2Zr$ | −4.04 | $H_{12}VHf_2Ag$ |
| −8.12 | $H_{12}VSc_2Ca$ | −4.02 | $H_{12}VHf_2Ge$ |
| −8.03 | $H_{12}VSc_2Hf$ | −3.96 | $H_{12}VTi_2Ni$ |
| −7.87 | $H_{12}VSc_2La$ | −3.82 | $H_{12}VTi_2Pd$ |
| −7.78 | $H_{12}VY_2Ba$ | −3.73 | $H_{12}VHf_2Sb$ |
| −7.36 | $H_{12}VHf_2Sc$ | −3.66 | $H_{12}VHf_2In$ |
| −7.10 | $H_{12}VSc_2Ba$ | −3.19 | $H_{12}VTi_2Cu$ |
| −7.02 | $H_{12}ScSc_2Sn$ | −3.03 | $H_{12}AlZr_2Sn$ |
| −6.77 | $H_{12}TiSc_2Sn$ | −2.93 | $H_{12}VTi_2Ag$ |
| −6.65 | $H_{12}LiTi_2Ti$ | −2.74 | $H_{12}VTi_2Cd$ |
| −6.57 | $H_{12}VZr_2La$ | −2.73 | $H_{12}CrTi_2Pd$ |
| −5.97 | $H_{12}TiTi_2V$ | −2.67 | $H_{12}LiTi_2Sn$ |
| −5.81 | $H_{12}AlZr_2Ti$ | −2.66 | $H_{12}CrHf_2Sb$ |
| −5.73 | $H_{12}VY_2Hg$ | −2.04 | $H_{12}CrTi_2Sn$ |
| −5.53 | $H_{12}VZr_2Ba$ | −1.85 | $H_{12}CrTi_2Ag$ |
| −5.25 | $H_{12}TiHf_2Au$ | −1.76 | $H_{12}CrTi_2As$ |
| −5.19 | $H_{12}VSc_2Cd$ | −1.60 | $H_{12}CrTi_2Au$ |
| −5.09 | $H_{12}VSc_2Hg$ | −1.51 | $H_{12}CrTi_2Sb$ |
| −5.00 | $H_{12}VZr_2Rb$ | −1.50 | $H_{12}CrTi_2In$ |

TABLE IV. List of the 62 kinds of the (12-1-3-1)-type hydrides which have the SEFs between −10.00 eV/f.u and 0.00 eV/f.u. and no spin polarization. The hydrides show the dynamical stabilities in NVTMDs.

| SEFs (eV/f.u.) | Material names | SEFs (eV/f.u.) | Material names |
|---|---|---|---|
| −4.88 | $H_{12}LiTc_3La$ | −2.27 | $H_{12}NaTc_3Sr$ |
| −4.62 | $H_{12}TiNi_3Ca$ | −2.25 | $H_{12}LiRe_3Ba$ |
| −4.58 | $H_{12}LiTc_3Sr$ | −2.19 | $H_{12}ScCu_3Ba$ |
| −4.51 | $H_{12}LiTc_3Ba$ | −2.13 | $H_{12}LiAl_3Rb$ |
| −4.39 | $H_{12}TiNi_3K$ | −1.98 | $H_{12}LiOs_3Ca$ |
| −4.16 | $H_{12}BeTc_3Sr$ | −1.90 | $H_{12}AlW_3La$ |
| −4.10 | $H_{12}TiPd_3Sr$ | −1.89 | $H_{12}BeRu_3Cs$ |
| −4.08 | $H_{12}BeTc_3La$ | −1.87 | $H_{12}BeTc_3Rb$ |
| −4.04 | $H_{12}TiPd_3Cs$ | −1.68 | $H_{12}LiAl_3K$ |
| −3.96 | $H_{12}BeTc_3Ba$ | −1.66 | $H_{12}BeRe_3Ba$ |
| −3.88 | $H_{12}TiPd_3Rb$ | −1.65 | $H_{12}LiRe_3Ca$ |
| −3.82 | $H_{12}LiMn_3Sr$ | −1.51 | $H_{12}NaAl_3Cs$ |
| −3.78 | $H_{12}MgTc_3Sr$ | −1.29 | $H_{12}ScCu_3Sr$ |
| −3.72 | $H_{12}AlMo_3La$ | −1.22 | $H_{12}NaAl_3Rb$ |
| −3.69 | $H_{12}ZnRu_3Sr$ | −1.15 | $H_{12}BeW_3Ba$ |
| −3.56 | $H_{12}VNi_3Cs$ | −1.04 | $H_{12}LiOs_3K$ |
| −3.55 | $H_{12}ScAl_3Rb$ | −0.96 | $H_{12}NaOs_3Ba$ |
| −3.48 | $H_{12}LiMn_3Ba$ | −0.93 | $H_{12}CuOs_3Ba$ |
| −3.37 | $H_{12}TiPd_3K$ | −0.84 | $H_{12}ScAl_3Hg$ |
| −3.25 | $H_{12}CuRu_3La$ | −0.79 | $H_{12}NaAl_3K$ |
| −3.19 | $H_{12}CuRu_3Sr$ | −0.74 | $H_{12}CuOs_3Sr$ |
| −3.15 | $H_{12}ZnTc_3Sr$ | −0.71 | $H_{12}CuRe_3La$ |
| −3.04 | $H_{12}LiOs_3Ba$ | −0.61 | $H_{12}NaOs_3Sr$ |
| −2.99 | $H_{12}CuTc_3La$ | −0.52 | $H_{12}MgOs_3Rb$ |
| −2.62 | $H_{12}BeRu_3Rb$ | −0.46 | $H_{12}BeOs_3K$ |
| −2.45 | $H_{12}AlMo_3Ca$ | −0.41 | $H_{12}MgOs_3K$ |
| −2.41 | $H_{12}NaTc_3Ba$ | −0.40 | $H_{12}LiOs_3Cs$ |
| −2.36 | $H_{12}LiAl_3Cs$ | −0.38 | $H_{12}BeOs_3Rb$ |
| −2.35 | $H_{12}CuRu_3Ca$ | −0.31 | $H_{12}ScAg_3Ba$ |
| −2.33 | $H_{12}ZnTc_3Ca$ | −0.27 | $H_{12}MgOs_3Cs$ |
| −2.32 | $H_{12}LiRe_3Sr$ | −0.13 | $H_{12}ScAl_3Cd$ |

TABLE V. List of the 36 kinds of the (12-1-3-1)-type hydrides which have the SEFs between −10.00 eV/f.u and 0.00 eV/f.u. and spin polarizations. The hydrides show the dynamical stabilities in NVTMDs.

| SEFs (eV/f.u.) | Material names | SEFs (eV/f.u.) | Material names |
|---|---|---|---|
| −6.10 | $H_{12}ScNi_3Ba$ | −3.20 | $H_{12}ZnTc_3Ba$ |
| −5.78 | $H_{12}TiCo_3Ba$ | −3.13 | $H_{12}ZnTc_3La$ |
| −5.43 | $H_{12}LiRu_3Sr$ | −2.93 | $H_{12}ZnV_3Ba$ |
| −4.74 | $H_{12}TiNi_3Rb$ | −2.72 | $H_{12}LiRu_3Cs$ |
| −4.62 | $H_{12}TiNi_3Cs$ | −2.66 | $H_{12}CuTc_3Sr$ |
| −4.61 | $H_{12}LiRu_3Ca$ | −2.65 | $H_{12}CuTc_3Ba$ |
| −4.29 | $H_{12}LiMn_3La$ | −2.60 | $H_{12}NaTc_3La$ |
| −4.17 | $H_{12}AlTc_3Ba$ | −2.43 | $H_{12}ZnMn_3La$ |
| −3.95 | $H_{12}LiFe_3Ba$ | −2.12 | $H_{12}VPd_3K$ |
| −3.80 | $H_{12}MgTc_3La$ | −1.92 | $H_{12}NaMn_3La$ |
| −3.64 | $H_{12}ScCr_3Ba$ | −1.65 | $H_{12}ZnCr_3Sr$ |
| −3.62 | $H_{12}VNi_3Rb$ | −1.49 | $H_{12}AlW_3Ba$ |
| −3.61 | $H_{12}ScMn_3Cs$ | −1.35 | $H_{12}ScAl_3I$ |
| −3.51 | $H_{12}LiRu_3K$ | −1.33 | $H_{12}CuRu_3K$ |
| −3.41 | $H_{12}LiRu_3Rb$ | −1.21 | $H_{12}MgRe_3Ba$ |
| −3.34 | $H_{12}MgMn_3Ba$ | −1.21 | $H_{12}CuCr_3Ba$ |
| −3.23 | $H_{12}AlMo_3Sr$ | −1.12 | $H_{12}CuCr_3Sr$ |
| −3.22 | $H_{12}VNi_3K$ | −0.79 | $H_{12}TiNi_3In$ |

TABLE VI. Pseudoatomic orbital basis functions.

| Atom | Quick Basis | Standard Basis | Atom | Quick Basis | Standard Basis |
|---|---|---|---|---|---|
| H | H5.0-s2 | H6.0-s2p1 | Rb | Rb11.0-s2p2d1 | Se11.0-s3p2d2 |
| Li | Li8.0-s3p1 | Li8.0-s3p2 | Sr | Sr10.0-s2p2d1 | Se10.0-s3p2d2 |
| Be | Be7.0-s2p1 | Be7.0-s2p2 | Y | Y10.0-s3p2d1 | Y10.0-s3p2d2 |
| B | B7.0-s2p2 | B7.0-s2p2d1 | Zr | Zr7.0-s3p2d1 | Zr7.0-s3p2d2 |
| C | C6.0-s2p2 | C6.0-s2p2d1 | Nb | Nb7.0-s3p2d1 | Nb7.0-s3p2d2 |
| N | N6.0-s2p2 | N6.0-s2p2d1 | Mo | Mo7.0-s3p2d1 | Mo7.0-s3p2d2 |
| O | O6.0-s2p2 | O6.0-s2p2d1 | Tc | Tc7.0-s3p2d1 | Tc7.0-s3p2d2 |
| Na | Na9.0-s3p2 | Na9.0-s3p2d1 | Ru | Ru7.0-s3p2d1 | Ru7.0-s3p2d2 |
| Mg | Mg9.0-s2p2 | Mg9.0-s3p2d1 | Rh | Rh7.0-s3p2d1 | Rh7.0-s3p2d2 |
| Al | Al7.0-s2p1d1 | Al7.0-s2p2d1 | Pd | Pd7.0-s3p2d1 | Pd7.0-s3p2d2 |
| Si | Si7.0-s2p1d1 | Si7.0-s2p2d1 | Ag | Ag7.0-s3p2d1 | Ag7.0-s3p2d2 |
| P | P7.0-s2p2d1 | P7.0-s2p2d1f1 | Cd | Cd7.0-s3p2d1 | Cd7.0-s3p2d2 |
| S | S7.0-s2p2d1 | S7.0-s2p2d1f1 | In | In7.0-s3p2d1 | In7.0-s3p2d2 |
| K | K10.0-s3p2 | K10.0-s3p2d1 | Sn | Sn7.0-s3p2d1 | Sn7.0-s3p2d2 |
| Ca | Ca9.0-s3p2 | Ca9.0-s3p2d1 | Sb | Sb7.0-s3p2d1 | Sb7.0-s3p2d2 |
| Sc | Sc9.0-s2p2d1 | Sc9.0-s3p2d1 | Te | Te7.0-s3p2d2 | Te7.0-s3p2d2f1 |
| Ti | Ti7.0-s2p2d1 | Ti7.0-s3p2d1 | I | I7.0-s3p2d2 | I7.0-s3p2d2f1 |
| V | V6.0-s2p2d1 | V6.0-s3p2d1 | Cs | Cs12.0-s3p2d1 | Cs12.0-s3p2d2 |
| Cr | Cr6.0-s2p2d1 | Cr6.0-s3p2d1 | Ba | Ba10.0-s3p2d1 | Ba10.0-s3p2d2 |
| Mn | Mn6.0-s2p2d1 | Mn6.0-s3p2d1 | La | La8.0-s3p2d1f1 | La8.0-s3p2d2f1 |
| Fe | Fe5.5H-s2p2d1 | Fe5.5H-s3p2d1 | Hf | Hf9.0-s3p2d2 | Hf9.0-s3p2d2f1 |
| Co | Co6.0H-s2p2d1 | Co6.0H-s3p2d1 | Ta | Ta7.0-s3p2d2 | Ta7.0-s3p2d2f1 |
| Ni | Ni6.0H-s2p2d1 | Ni6.0H-s3p2d1 | W | W7.0-s3p2d2 | W7.0-s3p2d2f1 |
| Cu | Cu6.0H-s2p2d1 | Cu6.0H-s3p2d1 | Re | Re7.0-s3p2d2 | Re7.0-s3p2d2f1 |
| Zn | Zn6.0H-s2p2d1 | Zn6.0H-s3p2d1 | Os | Os7.0-s3p2d2 | Os7.0-s3p2d2f1 |
| Ga | Ga7.0-s2p2d1 | Ga7.0-s3p2d2 | Ir | Ir7.0-s3p2d2 | Ir7.0-s3p2d2f1 |
| Ge | Ge7.0-s2p1d1 | Ge7.0-s3p2d2 | Au | Au7.0-s3p2d2 | Au7.0-s3p2d2f1 |
| As | As7.0-s3p2d1 | As7.0-s3p2d2 | Hg | Hg8.0-s3p2d2 | Hg8.0-s3p2d2f1 |
| Se | Se7.0-s3p2d1 | Se7.0-s3p2d2 | | | |
